# Supplementary material for: A strong loophole-free test of local realism
Source: arXiv:1511.03189 ancillary file (2016-09-06)
Supplement: Supplementary file 1 [file LHFSupplementary.pdf]

# Supplemental Material: A strong loophole-free test of local realism

Lynden K. Shalm,<sup>1</sup> Evan Meyer-Scott,<sup>2</sup> Bradley G. Christensen,<sup>3</sup> Peter Bierhorst,<sup>1</sup> Michael A. Wayne,<sup>3,4</sup> Martin J. Stevens,<sup>1</sup> Thomas Gerrits,<sup>1</sup> Scott Glancy,<sup>1</sup> Deny R. Hamel,<sup>5</sup> Michael S. Allman,<sup>1</sup> Kevin J. Coakley,<sup>1</sup> Shellee D. Dyer,<sup>1</sup> Carson Hodge,<sup>1</sup> Adriana E. Lita,<sup>1</sup> Varun B. Verma,<sup>1</sup> Camilla Lambrocco,<sup>1</sup> Edward Tortorici,<sup>1</sup> Alan L. Migdall,<sup>4,6</sup> Yanbao Zhang,<sup>2</sup> Daniel R. Kumor,<sup>3</sup> William H. Farr,<sup>7</sup> Francesco Marsili,<sup>7</sup> Matthew D. Shaw,<sup>7</sup> Jeffrey A. Stern,<sup>7</sup> Carlos Abellán,<sup>8</sup> Waldimar Amaya,<sup>8</sup> Valerio Pruneri,<sup>8,9</sup> Thomas Jennewein,<sup>2,10</sup> Morgan W. Mitchell,<sup>8,9</sup> Paul G. Kwiat,<sup>3</sup> Joshua C. Bienfang,<sup>4,6</sup> Richard P. Mirin,<sup>1</sup> Emanuel Knill,<sup>1</sup> and Sae Woo Nam<sup>1</sup>

<sup>1</sup>*National Institute of Standards and Technology, 325 Broadway, Boulder, CO 80305, USA*

<sup>2</sup>*Institute for Quantum Computing and Department of Physics and Astronomy,  
University of Waterloo, 200 University Ave West, Waterloo, Ontario, Canada, N2L 3G1*

<sup>3</sup>*Department of Physics, University of Illinois at Urbana-Champaign, Urbana, IL 61801, USA*

<sup>4</sup>*National Institute of Standards and Technology, 100 Bureau Drive, Gaithersburg, MD 20899, USA*

<sup>5</sup>*Département de Physique et d'Astronomie, Université de Moncton, Moncton, New Brunswick E1A 3E9, Canada*

<sup>6</sup>*Joint Quantum Institute, National Institute of Standards and Technology and University of Maryland,  
100 Bureau Drive, Gaithersburg, Maryland 20899, USA*

<sup>7</sup>*Jet Propulsion Laboratory, California Institute of Technology, 4800 Oak Grove Drive, Pasadena, CA 91109*

<sup>8</sup>*ICFO – Institut de Ciències Fotoniques, The Barcelona Institute  
of Science and Technology, 08860 Castelldefels (Barcelona), Spain*

<sup>9</sup>*ICREA – Institució Catalana de Recerca i Estudis Avançats, 08015 Barcelona, Spain*

<sup>10</sup>*Quantum Information Science Program, Canadian Institute for Advanced Research, Toronto, ON, Canada*

(Dated: November 21, 2015)

## I. METHODOLOGY FOR STATISTICAL INFERENCE AND HYPOTHESIS TESTING

### A. Memory-Robust Statistics

We use statistical hypothesis testing to draw inferences from our data, where the null hypothesis is that nature respects local realism. Our analysis assumes that our experimental apparatus functions correctly as described elsewhere in this manuscript. A test statistic (a real-valued function of the data) is computed for which the probability of seeing sufficiently large values is improbable under the null hypothesis, so extremely large values of the test statistic can be interpreted as evidence against local realism. In particular, the “p-value” is the maximum probability, under the null hypothesis, of seeing a test statistic as or more extreme than the experimentally observed value [S1]. The smaller the p-value, the more compelling the evidence against local realism.

Statistical methods often make an assumption that successive experimental trials are independent and identically distributed (i.i.d.). However, the i.i.d. assumption does not hold in real experiments, which are not perfectly stable. It is also possible that the local hidden variables have memory of previous trials and will attempt to use that information to violate a Bell inequality. Assuming i.i.d. behavior opens the “memory loophole” [S2]. To rule out local hidden variable theories exploiting the memory loophole, one must use statistics that are robust to memory effects [S2, S3]. In our experiment no photons are detected during a large number of trials, and these trials contribute little to the Bell violation. For such experiments, two effective memory-robust statistical inference methods are the prediction-based-ratio (PBR) protocol [S4, S5] and a martingale method based on a version of the CH inequality, which uses a binomially distributed test statistic [S6]. A single analysis method should be chosen in advance to determine the reported p-value, because if multiple analyses are performed and only the best p-value is reported, this overstates the confidence in the result.

The PBR protocol is powerful in that it provides an asymptotically optimal p-value bound in a stable experiment, but it can require a large number of experimental trials before converging at this optimal rate. Because the experiment was calibrated to maximize violation of the CH inequality, we used the binomial method of [S6]. (Preliminary tests of the PBR protocol, performed after the binomial method analysis was complete, suggest that similar p-value upper-bounds can be obtained using the PBR protocol.) Our test statistic is based on the following version of the CH inequality:

$$P(++ | ab) - P(+0 | ab') - P(0+ | a'b) - P(++ | a'b') \leq 0. \quad (\text{S1})$$

In the above,  $P(xy | zw)$  is the probability that Alice records outcome  $x$  and Bob records outcome  $y$  when the respective settings are  $z$  and  $w$ . The above inequality is a direct consequence of the assumption of local realism,

though it can also be derived from the original CH inequality [S7] by noting that

$$\begin{aligned} P(\text{Alice Single Count} \mid a) &= P(++ \mid ab') + P(+0 \mid ab') \\ P(\text{Bob Single Count} \mid b) &= P(++ \mid a'b) + P(0+ \mid a'b), \end{aligned}$$

which follow from the no-signaling assumption that Alice's outcome probabilities are independent of Bob's setting choice. No-signaling is itself a consequence of the local realism assumption. Equation (S1) is the form of the Clauser-Horne inequality used by Eberhard in [S8] with a slight modification as was performed to obtain equation (4) in [S9].

In an experiment with equiprobable measurement settings, equation (S1) implies that under local realism, the probability of getting outcome  $++ab$  is less than or equal to the sum of the probability of getting any of the three outcomes  $+0ab'$ ,  $0+a'b$ , or  $++a'b'$ . For a given data set and using a given set of downconversion slots, let  $\mathcal{T} = (T_k)$  be the sequence of all trial outcomes (both settings and measurement results) that have outcomes in the set  $\{++ab, +0ab', 0+a'b, ++a'b'\}$ . Let  $N_\chi$  be a positive integer chosen by the experimenter (as explained below). Let  $\chi = (T_k)_{k=1}^{N_\chi}$  denote the subsequence of trial outcomes taken from  $\mathcal{T}$  starting at the beginning and stopping at  $N_\chi$ . We define the sequence  $\mathcal{J} = (J_k)_{k=1}^{N_\chi}$ , where

$$J_k = \begin{cases} +1, & \text{if } T_k = ++ab \\ -1, & \text{if } T_k \neq ++ab. \end{cases}$$

We now define the test statistic to be  $N_S$  the number of elements of  $\mathcal{J}$  that equal +1.

It was shown in [S6] that under local realism, the sequence  $\mathcal{J}$  is a supermartingale and that

$$P(\text{at least } N_S \text{ of the elements of } \mathcal{J} \text{ equal } +1) \leq P(B_{N_\chi} \geq N_S), \quad (\text{S2})$$

where  $B_{N_\chi}$  is a binomial random variable corresponding to  $N_\chi$  trials with a probability of success 1/2. These results hold for general local hidden variable theories that are allowed memory, and the bound is tight in the sense that there are local hidden variable theories that achieve equality in (S2). Thus to compute a p-value, after the occurrence of a fixed number  $N_\chi$  of trials with outcomes in the sequence  $\mathcal{T}$  one counts the number  $N_S$  of  $++ab$  outcomes within this set and the p-value is then the probability of getting  $N_S$  or more “successes” out of  $N_\chi$  trials of a binomial random variable with probability of success 1/2.

## B. Protocols to guard against p-value hacking

For the p-values from this statistical procedure to be valid,  $N_\chi$  must be chosen using information available in advance of the experimental run. Running the experiment for a fixed amount of time and then computing the p-value for the entire sequence  $\mathcal{T}$  requires an assumption that no local realistic theory could stop the source. If a lucky fluctuation in the nonlocal direction occurs, an adversarial local realistic system with memory could stop producing outcomes that would be in  $\mathcal{T}$ —thus “locking in” the fluctuation.

To remove the need to make such an assumption, a small portion from the beginning of each dataset was used as a training set to estimate the fraction  $f$  of trials that will be in the sequence  $\mathcal{T}$ . (Different estimates of  $f$  were determined for each set of slots to be analyzed and for each data set that was analyzed.) We then set  $N_\chi = 0.9rf$ , where  $r$  was the number of trials remaining in the dataset after the training set is removed, and the scale factor of 0.9 was a chosen conservatively so that the probability of running out of trials in  $\mathcal{T}$  before reaching  $N_\chi$  in the run would be small. The p-value was determined using only the first  $N_\chi$  from the sequence  $\mathcal{T}$ . All trials after this cut point were discarded. If the  $N_\chi$  estimate had been too high, more data would have had to have been taken to complete the run, but this did not occur for any of the experimental runs analyzed here.

Here we present an example, taken from the data in the paper, that illustrate the dangers of not using a well-defined stopping criteria. In Fig. (S1) the accumulated p-value as a function of trial number is shown for the photons arriving in slot five of the data run reported in the main paper. To obtain the lowest p-value, we could stop after 63 583 981 trials (approximately 642s) and discard the rest of the trials. This yields a p-value that is nearly two orders of magnitude lower than the p-value computed at our  $N_\chi$  stopping criterion that is chosen blind. By repeating this process using different test statistics, optimizing on stopping criteria, and discarding entire data runs it is possible to end up with p-values that appear to be significant but are the result of statistical fluctuations that have been amplified. This is colloquially referred to as “fishing for correlations” or “p-value hacking.” To avoid these issues, well-defined statistical procedures should be established before the data is analyzed.

In our experiment, each experimental run was carried out for a fixed duration that was established before data taking began. During data taking various parameters were monitored, such as the mode-locking stability of the laser,

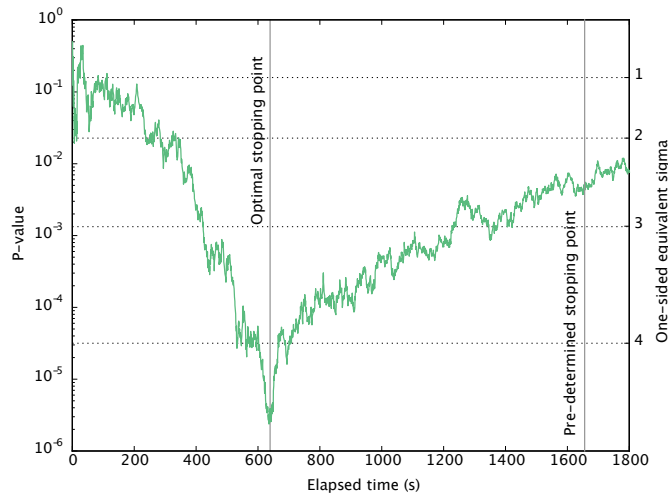

FIG. S1. Accumulated p-value over time for photons arriving in slot 4 (from the data reported in the main manuscript). The accumulated p-value changes over the course of the experimental run. Using only the first 641 s worth of data yields a p-value that is approximately two orders of magnitude smaller than if we use the stopping criterion chosen before the analysis started. The change in the p-value could be due to statistical fluctuations or experimental instabilities. However, not using well defined stopping criteria (or a hypothesis test robust to stopping criteria) can lead to statistical fluctuations being treated as significant results. This amplification of the significance of statistical fluctuations can also occur if the test static is optimized over the same data it will test. Engaging in these practices is known as “p-value hacking.” In a Bell test, analysis protocols need to be established in advance to avoid accidental p-value hacking.

the count rates, and a rough estimate of the Bell violation, but the person who applied the hypothesis test to the data was not involved in the data taking. We also took one data run that was completely blind—nothing was monitored during the experiment. We will analyze that data in the future using different hypothesis test techniques that are under development.

### C. Accounting for predictability in settings probabilities

One cannot characterize the probability distribution of a physical RNG exactly, so we would like for our statistical analysis to be robust to small deviations from equiprobability of the measurement settings. We also acknowledge the possibility that for some trials, the true probability of certain settings could be more than  $1/2$ , whereas on other trials, it could be less than  $1/2$ . For a given trial, Alice’s and Bob’s measurement choices have “predictabilities”  $\mathcal{P}_A$  and  $\mathcal{P}_B$ , defined as  $\mathcal{P}_A = \max(p_a, p_{a'})$  and  $\mathcal{P}_B = \max(p_b, p_{b'})$ , where  $p_a$  is the probability that Alice chooses setting  $a$ ,  $p_b$  is the probability that Bob chooses setting  $b$ , and  $p_{x'} = 1 - p_x$  for  $x = a, b$  are the probabilities for Alice and Bob choosing settings  $a'$  and  $b'$  respectively. It is impossible to measure the predictabilities with statistical tests of Alice and Bob’s choices, because the predictabilities may change from trial to trial. However, as described in Section III A, by modeling and characterizing the random number generators, one may place an upper bound on predictabilities. We bound both Alice’s and Bob’s predictabilities using the parameter  $\epsilon \in [0, 1]$  such that  $\mathcal{P}_A$  and  $\mathcal{P}_B \leq (1 + \epsilon)/2$ . Computation of p-values when  $\epsilon \neq 0$  has been studied in [S10, S11]. In the following, we use the treatment of [S10]. As is intuitive, a small predictability would increase the maximum probability under LR that members of  $\mathcal{J}$  equal  $+1$  above  $1/2$ . To compute p-values, a small correction must be applied to (S2), where the success probability of the binomial random variable is slightly increased. Our statistical method is able to tolerate any predictability within a small range, even if that predictability is chosen in each trial by an adversary attempting to violate a Bell inequality using a LR system. We do assume that, given the predictability, Alice’s and Bob’s choices are independent.

To find the precise value of the correction, we recall that any local realistic distribution can be expressed as a convex combination of local deterministic distributions [S12], of which there are 16. Due to the linearity of expectation, for any fixed setting probability distribution  $E(J_k)$  will achieve its maximum value at one of these local deterministic distributions. We can thus examine the 16 local deterministic distributions individually to see which one gives the highest  $E(J_k)$  for any settings probability distribution that obeys the predictability bounds, and report this as the maximum expectation of  $J_k$  under LR. We are interested in  $P(J_k = +1)$  specifically; as this a monotone function of  $E(J_k)$ , we can optimize it directly.

Consider the local deterministic distribution that always results in a “+” count at both detectors. This will result in a  $\mathcal{T}$  event with probability  $p_a p_b + p_{a'} p_{b'}$ . Thus the probability of getting a  $++ab$  event *conditioned on the occurrence of a  $\mathcal{T}$  event* is

$$\frac{p_a p_b}{p_a p_b + p_{a'} p_{b'}}, \quad (\text{S3})$$

and this is the probability that  $J = +1$ . One can optimize expression (S3) over the space of feasible values for  $p_a$  and  $p_b$  by examining partial derivatives to find that the expression achieves a maximum on the boundary when  $p_a = p_b = 1/2 + \epsilon/2$ . As (S3) is equal to  $P(J = +1)$ , a few arithmetical manipulations reveal that

$$P(J = +1) \leq \frac{1}{2} + \frac{\epsilon}{1 + \epsilon^2} \quad (\text{S4})$$

for this local deterministic strategy. All of the other 15 local deterministic distributions obey the bound (S4), and so this can be used as the adjusted binomial distribution’s probability of success when calculating modified p-values that allow for a degree of uncertainty in the predictability.

## II. TIMING DIAGRAMS AND MEASUREMENTS

To verify that the events in our experiment satisfy all the necessary spacelike separations, we performed a series of measurements to determine the transit times and latencies of all critical elements of the experimental setup. The timing diagram in Fig. (S2) shows the main results of these measurements as four separate timelines. All four originate in the source lab, and two each terminate in Alice and Bob. For directly measured quantities, uncertainties are estimated as described in the sections below. For derived quantities, uncertainties of the measured quantities are added in quadrature; this assumes the measurement uncertainties are uncorrelated with one another.

### A. Optical time domain reflectometry (OTDR)

We employed single-photon optical time domain reflectometry (OTDR) to measure the transit time of light through all the optical fibers and some of the free-space optical paths in the experimental setup. Single-photon OTDR measures the round-trip times of photons after reflection off any partially reflecting surfaces, including the fiber end facets and the entrance and exit facets of the source crystal and the Pockels cells. To do this, a  $\approx 200$  ps laser pulse with  $\approx 1551$  nm center wavelength and  $\approx 13$  nm full-width-half-maximum bandwidth is coupled into fiber and sent through a circulator. The circulator’s sampling output travels through a short piece of fiber terminated with a standard (FC-PC) fiber connector. The reflection off this connector serves as a timing reference. A fiber from the setup is then connected to this output, and the difference between return time from the end of the fiber and the timing reference is taken as twice the transit time through the fiber.

These return times are measured at the output port of the circulator, where the reflected light is directed to a superconducting nanowire single-photon detector (SNSPD) system. Photon arrival times are measured by constructing a histogram of time delays between the signal and reference using time-tagging electronics (a four-channel HydraHarp 400 [S13]). Uncertainties are estimated from the measured widths of the histograms, and are dominated by the laser pulse duration and SNSPD timing jitter. As a result, the transit time of light through a fiber hundreds of meters long can be determined with very high precision. Uncertainties for the OTDR measurements reported here range from 60 ps to 160 ps. The laser is operated at a repetition rate of 20 kHz, to ensure that only one pulse transits the fiber under test at a time, enabling unambiguous identification of the source of each reflected laser pulse. The wavelengths of our entangled photons and sync telecom transmitter lie within the bandwidth of the test laser used here, and dispersion does not play a significant role in the wavelength dependence of the transit times over the lengths of fibers (each  $< 200$  m) used in the experiment.

The pulse 1 fiber transit times are found from two measurements each at Alice and Bob. Before installing the Pockels cell bridge at each location, we first splice a test fiber pigtail to the long fiber coming from the source lab. This allows us to measure the transit time through the long fiber all the way to the SPDC source crystal. Next, we break this splice, and splice the test pigtail onto the fiber going the other direction, through the Pockels cell bridge and on to the SNSPD detection system. Finally, this second splice is broken and the long fiber from the source is spliced directly to the input fiber going to the Pockels cell bridge. We find the transit time through the test fiber pigtail by measuring its length and using the manufacturer specified index of refraction (1.468). This delay is then subtracted from our other measurements to obtain the source-to-detector transit time.

## B. Electrical time domain reflectometry (TDR)

We used electrical time domain reflectometry (TDR) measurements to characterize some of the coaxial cable delays in our setup. A short ( $\approx 5$  ns) rise-time electrical pulse from an 80 MHz-bandwidth arbitrary waveform generator is sent into a comparator circuit that emits a sharper ( $\approx 1$  ns) rise-time electrical pulse. This pulse is split with a coaxial tee at the input to the four-channel time tagger. The output of this tee is sent to a reference coaxial cable with an open (unterminated) end. After recording the return time off the end of this reference cable, the cable to be tested is connected to the end of this reference cable, again with an unterminated end, and the return time is measured. The difference in these two return times yields twice the cable transit time. Uncertainties are estimated from the standard deviation of the histogram widths.

## C. Single-pass latency measurements with an oscilloscope

Some components and cables were measured in a single-pass configuration using a 1 GHz, 4 Gsamples/s oscilloscope. This technique is useful when a traveling signal is interrupted by active components that are not compatible with the TDR technique, such as amplifiers and comparators.

## D. Latency of electrical-to-optical and optical-to-electrical conversion in the sync broadcast

The synchronization signal from the source to Alice and Bob is broadcast using a 1550 nm-wavelength telecom laser and receiver. The laser is triggered by the electrical synchronization signal, converting this to an optical signal at the source that is split with a fiber beamsplitter and sent to Alice and Bob via dedicated optical fibers (different from those the entangled photons travel in). At each end, a telecom receiver converts this optical signal back to an electrical pulse that triggers the interface circuit to sample the random number generators and drive the Pockels cell. To measure the latencies of electrical-to-optical and optical-to-electrical conversion, we output the transmitter (E-O converter) directly to each of the receivers (O-E converters) through a short fiber patch cable. Subtracting the time delay introduced by this fiber, which we determine by measuring its length and using the manufacturer specified index of refraction (1.468), yields a combined latency of E-O plus O-E conversion of  $\tau_{EO} + \tau_{OE} = 12.39 \pm 0.10$  ns for Alice and  $12.48 \pm 0.10$  ns for Bob.

## E. Fast photodiode latency

Although not important to our determination of spacelike separations, we tested the latency of the fast Si photodiode (Picoquant TDA200 [S13]) used to generate the sync pulses by comparing its response to that of a fast InGaAs photodiode. The InGaAs photodiode (Thorlabs D400FC [S13]) has a specified bandwidth of 1 GHz and rise time of 100 ps. It consists of a DC-biased InGaAs photodiode whose output directly follows a short ( $\approx 5$  cm) trace on a printed circuit board to the center pin of the output coaxial connection, with no amplifiers or resonant circuits. Although we do not have a direct measure of the InGaAs photodiodes latency, we are confident it can be bounded to  $< 1$  ns. By placing each detector at the same location in the free-space beam at the output of an  $\approx 800$  nm-wavelength, 550 kHz repetition rate, cavity-dumped Ti:Sapphire laser, we find that the Si photodiode response is delayed  $\approx 0.6$  ns with respect to the InGaAs response as measured on the 1 GHz oscilloscope. We thus estimate the latency of the fast Si photodiode as  $1 \pm 1$  ns.

## F. SNSPD latency

We measured the latency of each SNSPD detection system by comparing its response to the same fast InGaAs photodiode described above. First, the arrival time of a pulse from the low-repetition rate,  $\approx 1551$  nm pulsed laser described above is measured relative to its sync pulse output using the four-channel time tagger. To find the earliest time the photodiode pulse rises out of the noise, we set the time tagger threshold at a low value of 37 mV (for a  $\approx 150$  mV amplitude pulse). Next, we move the output of this fiber into the free-space path of each bridge, after the Pockels cell and waveplates. To attenuate the signal from that required for triggering the fast InGaAs photodiode, we place the end of the fiber  $\approx 8$  cm from the fiber coupler. This allows the beam to diverge, so that only a small fraction of photons exiting this fiber are coupled to the SNSPD detector system, reducing the average flux to  $\ll 1$  photon per

pulse, to avoid pile-up in time-of-arrival measurements. The four-channel time tagger threshold is set to 400 mV for the SNSPD output, consistent with the threshold value used by the 16-channel time tagger (UQDevices Coincidence Logic Unit[S13]) in the Bell violation experiment. Subtracting off the free-space path, we measure system detection latencies of  $49.9 \pm 0.5$  ns for Alice and  $44.5 \pm 0.5$  ns for Bob.

The latency of each SNSPD detection system can be decomposed into four components: (1) the time required for a photon to transit the fiber from the optical bridge into the cryostat and to the SNSPD, (2) the internal latency of the SNSPD, (3) the time required for the raw electrical pulse from the detector to transit the coaxial cable out of the cryostat, and (4) the time required for this pulse to pass through the bias tee, amplifiers and comparator, and through an additional coaxial cable to the 16-channel time tagger. We measured processes (1) and (3) using OTDR and TDR, respectively. These measurements were performed with the detector cold, to account for any temperature dependence of the propagation delays through fiber or coaxial cables. Process (4) was measured with an oscilloscope, as described above in section II C. To simulate a raw, unamplified SNSPD pulse arriving at the bias tee, the output of an 80 MHz arbitrary waveform generator was sent through four 10 dB coaxial attenuators in series. The latency of each attenuator was measured individually with the oscilloscope, and the measurement was compensated for the total latency of the four attenuators in series.

Process (2), the internal SNSPD latency, is the elapsed time from when a photon is incident on the detector until the raw electrical pulse output from the detector to its coaxial cable reaches a sufficiently large amplitude that, when amplified, will exceed the 400 mV trigger level set in the time tagger. Subtracting the time required for processes (1), (3) and (4) from the total detector system latencies yields the detector's internal latency. Within our uncertainties ( $\pm 0.5$  ns), the SNSPD internal latency is indistinguishable from the latency of this fast InGaAs photodiode. Taking a conservative approach, we estimate the SNSPD internal latency as  $1 \pm 1$  ns each for the MoSi SNSPD at Alice and the WSi SNSPD at Bob.

### G. Pockels cell latency

We measure the latency of each Pockels cell by sending a continuous-wave, 1550 nm-wavelength alignment laser through the setup along the same beam path as the entangled photon pairs. This provides a finer sampling of the turn-on and turn-off times than the 12.607 ns period of the Ti:Sapphire laser allows. We define the turn-on latency of each Pockels cell as the elapsed time from when the high voltage (HV) enable pulse arrives at the Pockels cell until the Pockels cell retardation reaches 90% of the plateaued “on” value. Similarly, the turn-off latency is the time between when the high voltage disable pulse arrives at the Pockels cell and the retardation reaches a level 10% above the nominal “off” value. For Alice, the measured turn-on and turn-off latencies are  $29.5 \pm 1.6$  ns and  $27.2 \pm 1.6$  ns, respectively. For Bob, these values are  $24.3 \pm 1.6$  ns and  $26.0 \pm 1.6$  ns. These values are consistent with the manufacturer specification of  $\approx 24$  ns.

### H. Distance measurements

The detectors, cryostats, time taggers, and other devices all have finite sizes and complicated geometries. To account for this we define a 0.8 m radius region at Alice, Bob, and the source that encompasses all relevant devices. We consider the measurements and entangled pair production to occur at some point within this region at the relevant stations. Using a combination of surveying measurements and GPS measurements, we measure the distances between the centers of these regions with uncertainties of 20 cm each. To simplify the analysis, we round our total uncertainty in the positions of Alice, Bob, and the source to a radius of 1 m.

### I. Reconciling the timelines

The sync and pulse 1 timelines for Alice can be reconciled by comparing the arrival times of the sync pulse and the SNSPD output pulse at Alice's time tagger. We then work backward on each timeline to the last location shared between the sync pulse and pulse 1, which is the beamsplitter just after the Ti:Sapphire laser. Using the measured values in Fig. (S2), we find that pulse 1 arrives at this beamsplitter  $618.2 \pm 1.6$  ns after the sync pulse. Repeating the same procedure for Bob yields an almost identical time difference of  $618.4 \pm 1.6$  ns. The nearest integer multiple ( $\times 49$ ) of the Ti:Sapphire laser repetition time of 12.607 ns is 617.7 ns, in excellent agreement with these two independently measured values. The similarity of these three quantities serves as a self-consistency check, giving us additional confidence in all the measured values and uncertainties shown in the timing diagrams. This further substantiates our claims of spacelike separation in the Bell test experiment.

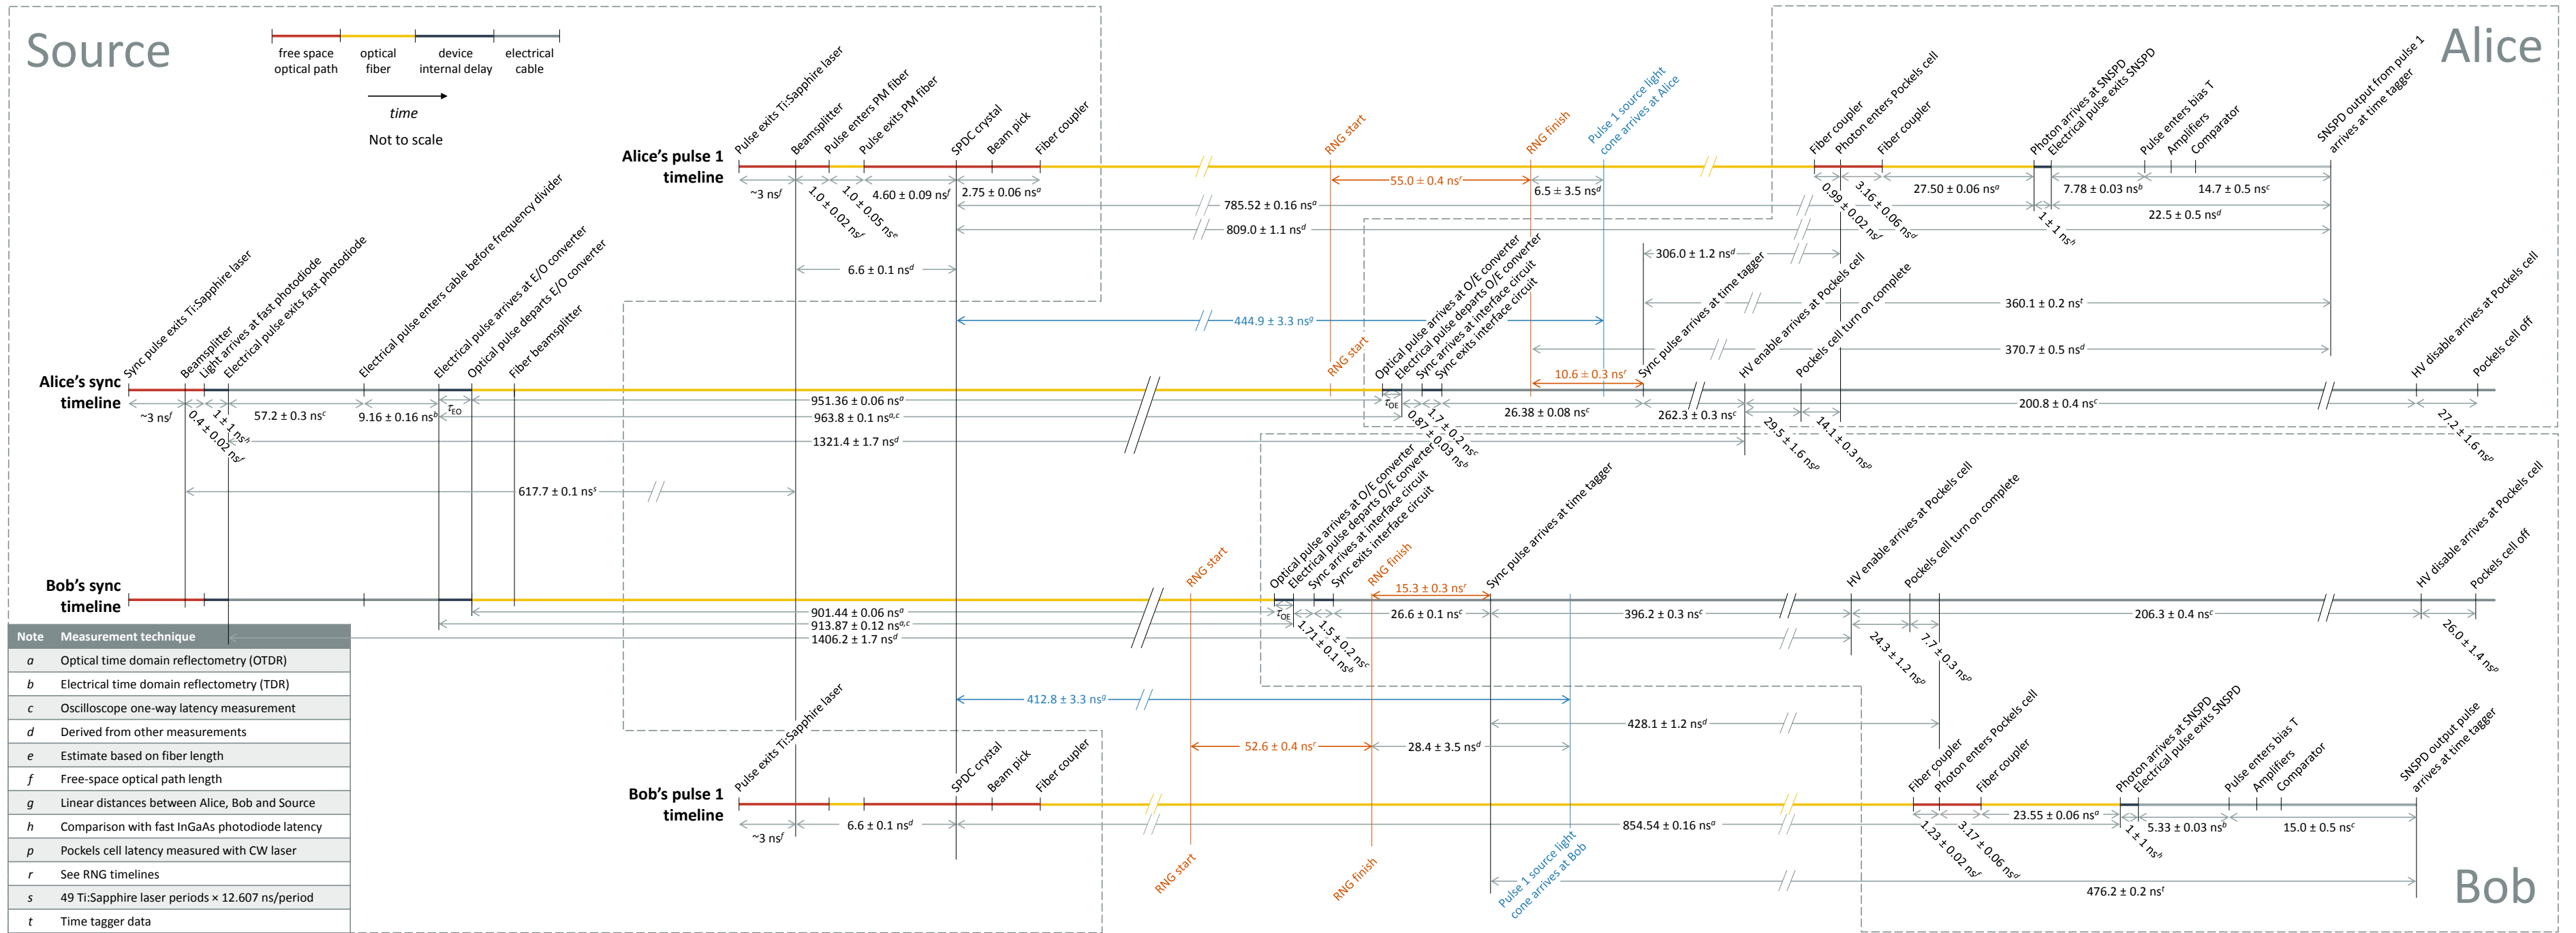

FIG. S2. Measured time delays and uncertainties in the experimental setup. Orange indicates random number generation (RNG) timing events, shown in detail in Fig. (S4). Light blue indicates events relevant to the forward light cone of pulse 1 from the source to Alice and Bob. Superscripts note how each value was determined, as listed in the table on the lower left and explained in the text. Abbreviations: PM fiber is polarization maintaining fiber, SPDC is spontaneous parametric downconversion, and HV is high voltage. The sums of the electrical-to-optical and optical-to-electrical latencies,  $\tau_{EO} + \tau_{OE}$ , are given in section IID.

### III. RANDOM BASIS CHOICE SETTINGS

To choose measurement settings, Alice and Bob each combines entropy from three qualitatively different sources to select the basis setting for the measurement. Two of these sources derive random bits from physical processes that are spacelike separated from both the remote measurement and from the entanglement generation. The third source combines a variety of pre-existing pseudorandom data derived from the digits of  $\pi$  and digital recordings of movies and television shows that are of a qualitatively different origin than the other two sources. For each trial, the sources are combined in a three-bit XOR, so that each basis setting fully depends on all three sources. The basis choice systems at Alice and Bob are of identical construction, except that different cultural pseudorandom data are used and the event timings are somewhat different.

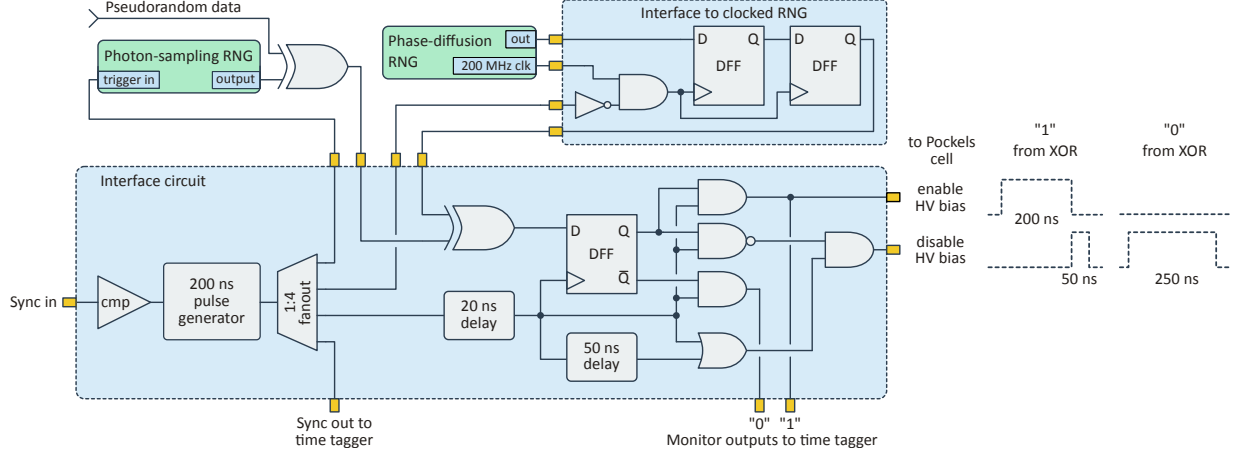

FIG. S3. Trial Measurement Settings. Measurement settings for each trial are implemented by XORing three random bit sources and applying the resulting setting to the Pockels cell driver. A high-speed comparator (cmp) detects the rising edge of the 99.1 kHz synchronization signal and triggers the generation of a 200 ns pulse. A gigahertz fanout produces four simultaneous replicas of this pulse: one triggers the PSRNG (cf. section IIIB), whose output is XORed with pseudorandom data (cf. section IIIC), one is sent to an interface circuit that latches a bit from the PDRNG (cf. section IIIA), one is sent to the time tagger as a temporal reference for the trial start, and one is used to set the state of the Pockels cell based on the XOR of all three RNGs. A delay of 20 ns accommodates latencies in the RNGs, coaxial connectors, and XOR chips, after which the output of the second XOR is sampled by a D flip-flop. The output of the DFF is sent through a set of discrete logic gates to generate the signals necessary for the double-push-pull Pockels cell driver [S13, S14].

#### A. Phase-diffusion random number generator (PDRNG)

One source of random bits is an accelerated laser phase-diffusion random number generator (PDRNG). The design, modeling, and testing of these devices is described in detail in [S15–S17]. The PDRNG at each measurement station continually generates “raw” bits  $d_i$  at a rate of 200 MHz, where  $i$  indexes the bits. The random signal is due to interference of macroscopic pulses of laser light with random phases acquired by spontaneous emission-driven phase diffusion in the time between pulses. Following the discussion in Section IC, the predictability  $\mathcal{P}_d$  of the raw bits, which is the larger of  $P(d=0)$  and  $P(d=1)$ , has an upper bound of  $\mathcal{P}_d \leq \frac{1}{2}(1 + \epsilon_{\max})$ , where  $\epsilon_{\max}$  is determined by comparing the measured strength of the  $\approx 1$  V peak-to-peak phase-diffusion signal against the measured  $\approx 10$  mV r.m.s. noise due to untrusted optical and electronic sources. Assuming the worst-case scenario of fully correlated, untrusted noises, we define  $\epsilon_{\max}$  to be the predictability error produced by a  $6\sigma$  fluctuation of the noise, so that  $\mathcal{P}_d$  exceeds  $\frac{1}{2}(1 + \epsilon_{\max})$  very rarely, with probability  $< 2 \times 10^{-9}$ . With this definition and the statistical metrology results,  $\epsilon_{\max} \leq 0.12$ .

Fast digital logic components perform a running parity calculation of  $x_i = d_i \oplus x_{i-1}$ , where  $x$  is the output signal. In this way  $x_i$  is the parity of  $d_i$  and thus aggregates randomness from all previous raw bits. All but the most recent  $k$  bits will, however, be in the past lightcone of the distant detection event. Assuming these older bits contribute nothing to the randomness of  $x$ , the predictability of the extracted bits is  $\mathcal{P}_x \leq \frac{1}{2}(1 + \epsilon_{\max}^k)$ .

We take the time at which the randomness is generated to be the 1 ns window preceding the rising edge of the pulse of injection current. Within this window, the phase diffusion is strongest and fully randomizes the phase; after this time, stimulated emission irreversibly amplifies the intra-cavity field to produce a macroscopic number of photons.

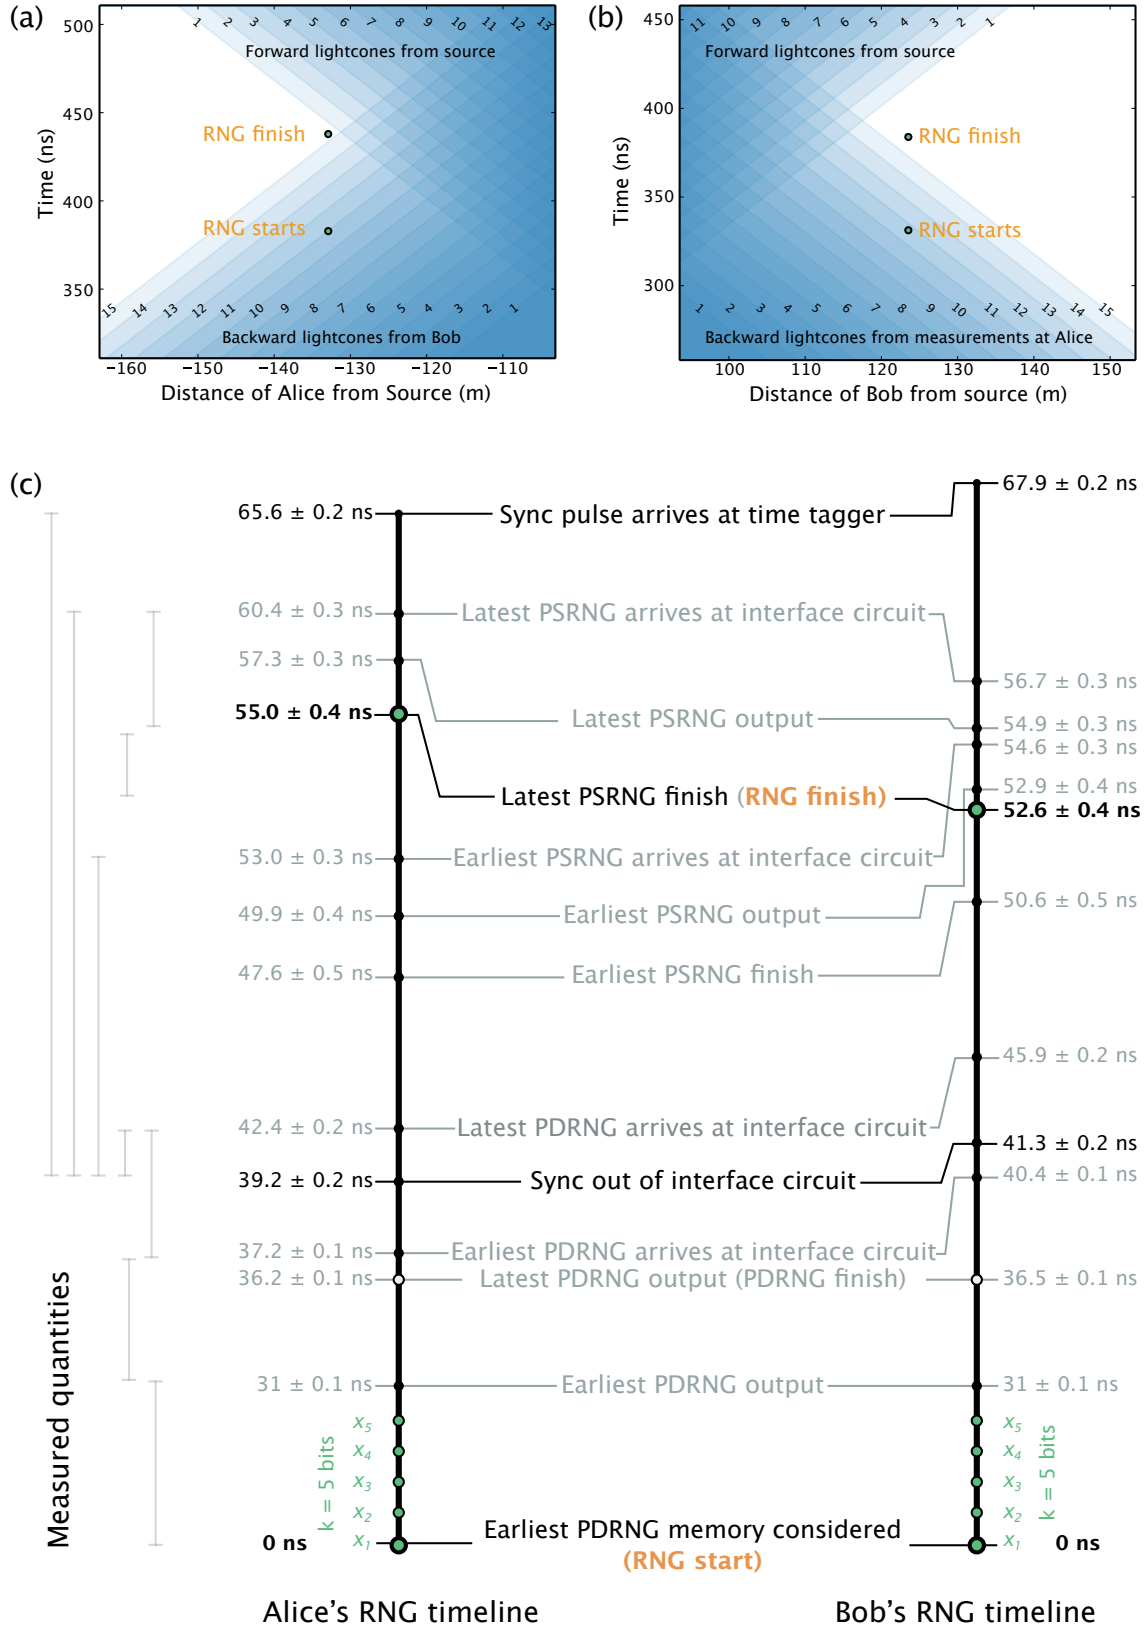

FIG. S4. (a) Minkowski diagram for events at Alice's random number generator and (b) Bob's random number generator. The forward and backward lightcones for different pulses are shown in light blue. (c) Timeline of events of Alices and Bobs random number generators are shown. The vertical bars on the left hand side indicate the timing differences that were physically measured in order to determine the event timing. Orange text indicate the time delays relevant to overall random number generator start and finish, and also appear in Fig. (S2).

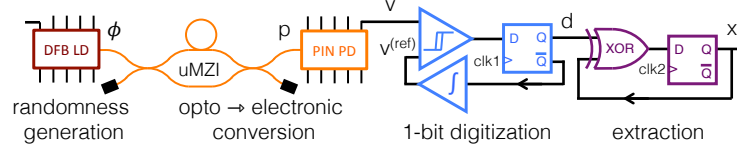

FIG. S5. Schematic of phase diffusion random number generator (PDRNG). Signal propagation is from left to right except on the lower lines, where it is right to left. DFB LD: distributed feedback laser diode, uMZI: unbalanced Mach-Zehnder interferometer, PIN PD: 10 Gbps linear photo-receiver,  $\triangleright$ : comparator,  $\triangleleft$ : integral feedback circuit, squares: D-type flip-flop, XOR: exclusive OR. The laser is pulsed at 5 ns intervals, creating a new bit of the sequence  $\{d_i\}$  with each pulse.  $\phi$ : phase of laser pulse, a variable randomized by spontaneous emission,  $v$ : analog voltage with  $\approx 1$  V range due to random laser phase and  $\approx 10$  mV noise due to electronics and laser amplitude noise,  $v^{(\text{ref})}$ : comparator reference voltage set by feedback from digitized values,  $d$ : digitized value, *i.e.* “raw bit”,  $x$ : result of running parity calculation and output of PDRNG.

These photons leave the laser cavity, experience interference in an interferometer, are detected, digitized, contributed to the parity, and output in the following 10 ns. A time  $t_{\text{PD}}$  is available for accumulation of  $k$  space-time separated PDRNG bits. This time is constrained by the requirements for achieving spacelike separation of the measurement choice from both the downconversion event and the remote measurement event. Considering the 5 ns pulse repetition period and the 11 ns time from production to availability,

$$k = \left\lfloor \frac{t_{\text{PD}} - 11 \text{ ns}}{5 \text{ ns}} \right\rfloor \quad (\text{S5})$$

where  $\lfloor y \rfloor$  indicates the largest integer smaller than  $y$ . Satisfying the spacelike separation constraints when seven pulses are aggregated in each trial allows for  $k = 5$ .

While statistical testing is not capable of certifying randomness, statistical tests nonetheless give some information about the quality of the raw bits and the efficacy of the extraction procedure. Prior to the experiment, the two PDRNGs were tested at  $k = 4$ , implemented by keeping only every fourth output bit, for which  $\epsilon_{\text{max}}^4 \leq 2.0 \times 10^{-4}$ . As described in [S17], we applied the test suites NIST SP800-22 [S18] and more extensively TestU01 Alphabit battery [S19], always finding results consistent with ideal randomness. One PDRNG was tested with a total of 464 Gbit of output, the other with a total of 171 Gbit. The largest files tested contained 64 Gbit of data. Using the statistical uncertainty of a test of this length, we obtain a  $1\sigma$  error bound of  $\mathcal{P} < \frac{1}{2}(1 + \frac{1}{\sqrt{64 \times 10^9}}) = \frac{1}{2}(1 + 4.0 \times 10^{-6})$ . The  $k = 4$  output passes the tests at this level of precision, suggesting that the statistical metrology results are quite conservative. We use the  $k = 4$  bound  $\epsilon_{\text{max}}^4 \leq 2.0 \times 10^{-4}$ , rather than the lower  $k = 5$  bound, to describe the experiment. With this value the RNGs excess predictability is small relative to  $\epsilon_p$  (c.f. Section III D) while being conservative relative to both the model-based predictions and the statistical testing.

We note that the randomness of laser phase diffusion is not restricted to quantum models. It is an experimental observation, repeated on many kinds of lasers, that the phase of a laser executes a diffusive motion proportional to the spontaneous emission rate. Spontaneous emission, by Einstein’s thermodynamic A and B coefficient argument, is a necessary accompaniment of stimulated emission, and thus of laser amplification [S20]. It would thus be difficult to exclude spontaneous emission, the archetype of a stochastic physical process, from the description of laser phase diffusion. We also note that a fully classical description of the laser behavior, in which a plasma of electrons careen around inside the semiconductor material and radiate into the cavity mode, would likely be chaotic, so that prediction of the future phase of the field would require an exponential precision in knowledge of the present conditions.

## B. Photon-sampling random number generator (PSRNG)

An additional source of random bits for the measurement choice in each trial is based on single-photon detection of optical states in the high-loss regime, a photon-sampling random number generator (PSRNG). Photodetection (or photoionization) with light attenuated to low mean-photon numbers is a probabilistic process. By sampling the output of a detector over an interval of time in which the optical-state and vacuum-state contributions are balanced, the detection probability can be set to 0.5 and used for random bit generation. This probability depends primarily on the amplitude of the attenuated optical state, as opposed to the PDRNG in section III A, in which randomness is generated from the phase of optical states.

The preparation and detection of the optical state is carried out in a fast, single-shot manner initiated by the receipt of a trigger. This allows us to generate a random bit on demand with low latency between trigger and output; a schematic of the PSRNG is shown in Fig. (S6). When triggered, a gain-switched vertical-cavity surface-emitting laser

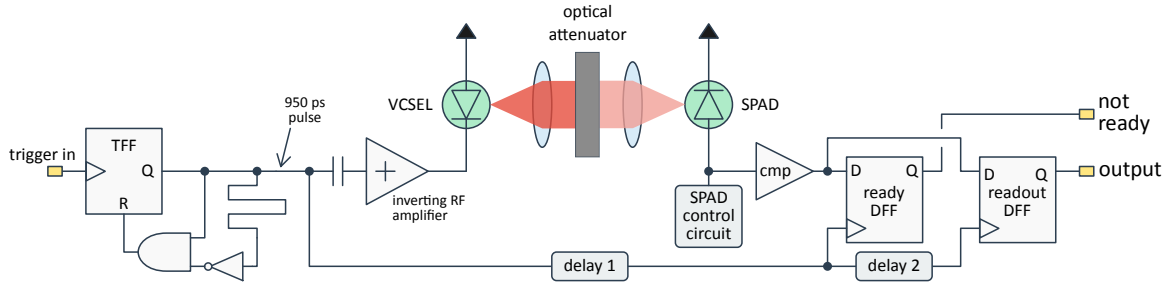

FIG. S6. Schematic of the photon-sampling random number generator. The PSRNG is triggered by the rising edge of the pulse, which clocks a fast resettable toggle flip-flop (TFF) and produces a 950 ps pulse that drives a gain-switched VCSEL. The optical output is strongly attenuated and focused on a single-photon avalanche diode (SPAD). An integrated high-speed comparator (cmp) provides low-latency readout of detections. The cmp output state is sampled by D flip flops (DFFs) at the start and the end of a time interval defined by fixed delays 1 and 2. The first, “ready” DFF indicates those rare instances when the RNG is not ready to produce a bit because it is recovering from a recent dark count, the “readout” DFF reports the measurement result.

(VCSEL) generates a  $\approx 1$  ns laser pulse that is attenuated and focused onto a single-photon avalanche photodiode (SPAD). Avalanche signals from the SPAD are detected by a high-speed comparator coupled directly to two flip flops. Additional circuitry (not shown) ensures that the comparator’s output stays at logical high for the entire  $\approx 55$  ns recovery time of the SPAD, during which the detector is disabled.

Output bit values are determined from whether or not a detection event occurred in an interval whose beginning and end are defined by the clocking of the two flip flops. A high-level output from the first flip flop indicates that at the start of the interval the SPAD was still disabled due to a dark-count event that occurred within the preceding  $\approx 55$  ns, meaning that the output bit for that trigger was determined as much as 55 ns earlier than expected. This “not ready” signal occurs at a rate of  $\approx 10^{-5}$  per trial. The second flip flop outputs a logic level determined by whether or not a detection occurred at some point during the measurement interval; no detection corresponds to a “0” while a detection corresponds to a “1”. The latency of the PSRNG, defined as the time between the earliest opportunity for optical emission from the VCSEL and the availability of the bit at the output of the readout DFF, has been measured to be as low as  $(2.4 \pm 0.2)$  ns. In the experiment, additional cable and on-board delays increased the total time between request and delivery of the random bit. For testing, the PSRNG was run continuously at a trigger rate of 100 kHz for 2.8 hours, and 1 Gbit of output bits with no post processing were recorded and analyzed using the NIST SP800-22 Statistical Test Suite for random number generators [S18]. Its output was found to pass all tests with a significance level  $\alpha = 0.01$ . Details about the operation and performance of this randomness source will be discussed in a future work. The timing of the PSRNGs relative to the PDRNGs is shown in Fig. S4.

### C. “Cultural” pseudorandom source

As a safeguard against potential systematic or conspiratorial effects, we took a series of measurements where the two physical random bits described above were combined through an XOR gate with a pre-determined string of pseudorandom bits. Both Alice’s and Bob’s pseudorandom bit strings are the result of XORing several files containing bits of movie files and the digits of  $\pi$ . To generate each string, we used an XOR to combine three different sets of numbers for each party. Each individual file was 1.5 Gbit long. For both Alice and Bob, two files were XORed with the file being read from start to finish, whereas a third file was read in reverse order. For each file of a show or movie, we used the middle 2/3 of the file in order to remove any headers and trailers in the data file.

To generate the file for Alice, we XORed the binary data string of “Back to the Future 1”, “Back to the Future 3” (which was used in reverse order), a concatenation of episodes of “Saved by the Bell” (see below), and a concatenation of  $1 \times 10^9$  digits of  $\pi$  after applying a modulo 2 operation with “Monty Python and the Holy Grail”. Alice’s total string passed every test in the NIST SP800-22 test suite [S18] except one of the 147 different non-overlapping template tests (95/100 of the bit streams still passed the NIST suite for the failed test). From this, the string appears largely aperiodic because the non-overlapping template tests check the file for any repeats of different aperiodic bit strings. The strings also passed the Dieharder tests [S21] and ENT tests [S22] with an average entropy for the whole file of 7.999999 bits/byte, verifying the file to be pseudorandom.

To generate the file for Bob, we XORed episodes of “Doctor Who” (which were all concatenated together), “Back to the Future 2”, and the concatenation of *Leonard Nimoy: Star Trek Memories* with episodes of “Star Trek” (this complete file was used in reverse order). Bob’s classical string passed every test in the NIST suite. It also passed all

of the Dieharder and ENT tests with an average entropy for the whole file of 7.999999 bits/byte, again verifying the file is pseudorandom.

These files were then used to generate a TTL signal from a data acquisition card. This bit stream was combined on a XOR gate with output of the PARNG before the XOR with the PDRNG to make the measurement setting choice at each measurement station.

List of content for Alice:

1. *Back to the Future*. Dir. Robert Zemeckis. Universal Studios, 1985.
2. *Back to the Future Part III*. Dir. Robert Zemeckis. Universal Studios, 1990.
3. Engel, Peter, and Tom Tenowich. "Dancing to the Max." *Saved by the Bell*. Dir. Don Barnhart. NBC. 20 Aug. 1989. Television.
4. Tenowich, Tom. "The Lisa Card." *Saved by the Bell*. Dir. Don Barnhart. NBC. 26 Aug. 1989. Television.
5. Tramer, Bennett. "The Gift." *Saved by the Bell*. Dir. Dennis Erdman. NBC. 8 Sept. 1989. Television.
6. Fink, Mark. "Fatal Distraction." *Saved by the Bell*. Dir. Gary Shimokawa. NBC. 9 Sept. 1989. Television.
7. Colleary, R. J. "Screech's Woman." *Saved by the Bell*. Dir. Gary Shimokawa. NBC. 16 Sept. 1989. Television.
8. Swerdlick, Michael. "Aloha Slater." *Saved by the Bell*. Dir. Don Barnhart. NBC. 23 Sept. 1989. Television.
9. Tramer, Bennett. "Miss Bayside." *Saved by the Bell*. Dir. Don Barnhart. NBC. 27 Oct. 1990. Television.
10. Balmagia, Larry. "The Babysitters." *Saved by the Bell*. Dir. Don Barnhart. NBC. 1 Dec. 1990. Television.
11. Tramer, Bennett. "Glee Club." *Saved by the Bell*. Dir. Don Barnhart. NBC. 23 Dec. 1990. Television.
12. Sachs, Jeffrey J., and Don Barnhart. "Date Auction." *Saved by the Bell*. NBC. 9 Nov. 1991. Television.
13. Tramer, Bennett. "Home for Christmas (Part 2)." *Saved by the Bell*. Dir. Don Barnhart. NBC. 14 Dec. 1991. Television.
14. Tenowich, Tom. "Student Teacher Week." *Saved by the Bell*. Dir. Don Barnhart. NBC. 12 Sept. 1992. Television.
15. Malman, Jeff, dir. "Screech Love." *Saved by the Bell*. NBC. 26 Oct. 1993. Television.
16. *Monty Python and the Holy Grail*. Dir. Terry Gilliam and Terry Jones. Perf. Graham Chapman. Ambassador Film Distributors, 1975. Film.

List of content for Bob:

1. Moffat, Steven. "The Eleventh Hour." *Dr. Who*. BBC. 3 Apr. 2010. Television.
2. Moffat, Steven. "The Time of the Angels." *Dr. Who*. Dir. Adam Smith. BBC. 24 Apr. 2010. Television.
3. Moffat, Steven. "Flesh and Stone." *Dr. Who*. Dir. Adam Smith. BBC. 1 May 2010. Television.
4. Moffat, Steven. "The Big Bang." *Dr. Who*. Dir. Toby Haynes. BBC. 26 June 2010. Television.
5. *Back to the Future Part II*. Dir. Robert Zemeckis. Universal Studios, 1989.
6. Logsdon, John, and Ryan Strober. *Star Trek: Beyond the Final Frontier*. Dir. John Logsdon. Prod. Paramount Pictures. The History Channel. 19 Feb. 2007. Television.
7. McGinn, Jim. *Leonard Nimoy: Star Trek Memories*. Dir. Kevin Curtis. Prod. Paramount Pictures. 1984. Television.

## D. Estimates of predictability

In our experiment each settings choice at Alice and Bob is determined by XORing three sources of random bits together. During the course of the experiment we observe that the fraction of trials for the “0” setting exceeds 0.5 by  $8.0 \times 10^{-5}$  and  $1.6 \times 10^{-5}$  at Alice and Bob respectively. However, it is possible that a local realistic model could be controlling the inputs of one or more of the random number generators used by Alice and Bob. In principle, the predictability of a random number generator cannot be measured through statistical tests, because their outputs can be made to appear random, unbiased, and independent by a local realistic system. However, using detailed physical models of the randomness processes and measurements of the random number generators themselves, one can develop estimates of the excess predictability present.

According to physical models described in section III A, the excess predictability of the PDRNG is  $\leq 2.0 \times 10^{-4}$  for  $k = 4$ , which is conservative relative to  $k = 5$ , the maximum  $k$  allowed by our spacelike separation constraints. The PDRNG is run asynchronously with respect to the rest of the experiment, so an interface board was designed to synchronize readout from the random number generator on demand. Through extensive testing after the data was taken, it was discovered that a combination of uncontrolled environmental variables and the synchronization board can introduce an unwanted bias up to  $(1.08 \pm 0.07) \times 10^{-4}$  and  $(0.81 \pm 0.02) \times 10^{-4}$  away from 1/2 for Alice and Bob, respectively. If we use this bias as a proxy for the excess predictability, this bias then corresponds to an excess predictability of approximately  $2 \times 10^{-4}$ . To be conservative, we grant a hypothetical local realistic system fifteen times this excess predictability,  $\epsilon_p = 3 \times 10^{-3}$  and adjust our p-values using this  $\epsilon_p$ .

Combining the random bits from the PDRNG with the output of the PSRNG and the cultural pseudorandom source should lower the excess predictability in our system. However, we note that taking  $\epsilon_p$  as the predictability of the PDRNG bits after synchronization, and making the nearly superdeterministic, paranoid, assumption that the hidden variable model can predict the PSRNG and cultural source with certainty, the observed Bell inequality violation is still strong.

## IV. ANALYSIS OF OTHER DATA SETS

### A. Description of other data sets

We recorded six data sets over two days using different experimental configurations that were analyzed. These six data sets will be made publicly available. We also took a blind data set that was not analyzed. Here is a description of each data set.

#### 1. Data sets using only the PDRNG and PSRNG XORed together (no cultural pseudorandom data).

*02\_54:* Stopping criteria was set to when Alice and Bob each collect approximately 15 GB of data. We noticed that the pump laser lost mode-locking toward the end of the run.

*03\_43:* After fixing the laser mode-locking, a new run was started. This run is shorter as one of the cryostats with the superconducting detectors warmed up. Data taking was then suspended until the following day once the cryostat had cooled down again.

*17\_04:* The system was realigned and a completely blind data run lasting 1 hour was taken. This file has not yet been processed or analyzed. Future work will report on optimal methods for conducting hypothesis tests on blind data.

*19\_45:* After the blind data run, some minor realignment of the system was carried out before starting this run. The stopping criteria was set at 30 minutes.

#### 2. Data sets using the PDRNG, PSRNG, and cultural pseudorandom source XORed together.

*XOR 1* Minor realignment was carried out before starting this data run. Stopping criteria was set at 30 minutes.

*XOR 2* Started a second data run shortly after *XOR 1*. No realignment performed. Stopping criteria was set at 30 minutes.

*XOR 3* System was realigned before the start of this data run. Stopping criteria was set at 30 minutes. This is the data set reported in the main manuscript.

## B. P-values

Table S-I reports p-values obtained from each data run. During analysis we can choose time windows that contribute to each trial of the experiment such that the windows correspond to different downconversion pulses, 15 of which arrive while the measurement settings are fixed. Each column of Table S-I shows p-values computed using time windows centered around pulse 6 and containing pulses listed in the column header. All sets of pulses in Table S-I maintain the spacelike separations required for a loophole-free test. For each data set, rows display the  $N_\chi$  cut point, the pre-determined number of trials with outcomes in the sequence  $\mathcal{T}$  used to compute the p-values;  $N_S$ , the number of trials in the first  $N_\chi$  elements of  $\mathcal{T}$  with outcome  $++ab$ ; and the p-values obtained under different values of  $\epsilon$ . We also report  $N_{\text{Total}}$ , the total number of trials for each data run, at the head of each sub-table. To aid the reader in calculating various Bell inequalities, we report all of the measurement settings and outcomes for the case with 5 aggregate pulses from the data set reported in the main manuscript (see Table S-II). This was the pulse combination that yielded the lowest p-value.

## C. Other diagnostic statistics

Other statistical tests were performed on the data to look for any anomalies that might raise questions about the validity of the experimental assumptions. For these tests we used standard statistical techniques and assumed the sources are independent and identically distributed (the i.i.d. assumption).

### 1. Independence of Alice's and Bob's settings.

Alice's probability of choosing  $a$  or  $a'$  should be independent of Bob's setting choice (and vice versa). We test this as a comparison of two proportions, with the null hypothesis being that Alice's probability of getting setting  $a$  when Bob gets  $b$  is the same as Alice's probability of getting setting  $a$  when Bob gets  $b'$ . As this is mathematically equivalent to the same test with Alice and Bob interchanged, there is only one test statistic for each experimental run. The p-values were 0.67, 0.04, 0.27, 0.37, 0.52, and 0.68, which appears consistent with a uniform distribution of p-values and gives us no reason to doubt the independence of Alice's and Bob's settings.

### 2. No signaling.

Alice's probability of seeing a “+” outcome should be independent of Bob's setting choice, and vice versa. If this were not to be the case, one party could use the setting choice to convey information to the other party faster than the speed of light, resulting in a type of nonlocality that is strictly stronger than what is possible under quantum mechanics. Given the spacelike separation of Alice and Bob, the presence of signaling effects in our data would be highly anomalous.

For a single experimental run, there are four independent signaling checks that can be performed: Bob's potential to signal Alice when Alice chooses  $a$ , Bob's potential to signal Alice when Alice chooses  $a'$ , and two symmetric ways for Alice to signal Bob. These notions can be formulated mathematically in terms of conditional probabilities. For instance, the statement that Bob cannot signal Alice when Alice chooses  $a$  can be formulated as the null hypothesis that  $P(+_A | ab) = P(+_A | ab')$ , and this equality can be tested as a comparison of two proportions. With 6 experimental runs, this would result in 24 independent p-values. We also checked the signaling behavior for five different pulse groupings—the four groupings in Table S-I along with pulse grouping 2-10. This leads to 120 p-values with some dependence between pulse groupings. The smallest observed p-value was 0.0017, which is not surprisingly small given the number of p-values computed. As shown in Table S-III, the distribution of the 120 p-values was also quite uniform across the range from 0 to 1. We thus see no evidence for the presence of anomalous signaling effects in the data.

TABLE S-I. Table of p-values testing LR.

| 02-54 (first run), $N_{\text{Total}} = 203,629,242$  |       |                       |                       |                       |
|------------------------------------------------------|-------|-----------------------|-----------------------|-----------------------|
| Pulses                                               | 6     | 5-7                   | 4-8                   | 3-9                   |
| $N_{\chi}$ Cut Point                                 | 2528  | 7659                  | 12753                 | 17854                 |
| $N_S$                                                | 1263  | 3842                  | 6460                  | 9057                  |
| $\epsilon = 0$ p-value                               | .5238 | .3920                 | .0708                 | .0263                 |
| $\epsilon = .0001$                                   | .5278 | .3987                 | .0739                 | .0280                 |
| $\epsilon = .001$                                    | .5637 | .4605                 | .1067                 | .0473                 |
| $\epsilon = .01$                                     | .8566 | .9300                 | .7848                 | .7685                 |
| 03-43 (second run), $N_{\text{Total}} = 107,032,197$ |       |                       |                       |                       |
| Pulses                                               | 6     | 5-7                   | 4-8                   | 3-9                   |
| $N_{\chi}$ Cut Point                                 | 1213  | 3678                  | 6192                  | 8668                  |
| $N_S$                                                | 618   | 1893                  | 3190                  | 4471                  |
| $\epsilon = 0$ p-value                               | .2638 | .0388                 | .0087                 | .0017                 |
| $\epsilon = .0001$                                   | .2661 | .0399                 | .0091                 | .0018                 |
| $\epsilon = .001$                                    | .2871 | .0502                 | .0132                 | .0030                 |
| $\epsilon = .01$                                     | .5259 | .2906                 | .2110                 | .1422                 |
| 19-45 (third run), $N_{\text{Total}} = 182,560,876$  |       |                       |                       |                       |
| Pulses                                               | 6     | 5-7                   | 4-8                   | 3-9                   |
| $N_{\chi}$ Cut Point                                 | 2455  | 7304                  | 11891                 | 16648                 |
| $N_S$                                                | 1246  | 3692                  | 6016                  | 8465                  |
| $\epsilon = 0$ p-value                               | .2337 | .1776                 | .0996                 | .0148                 |
| $\epsilon = .0001$                                   | .2368 | .1821                 | .1035                 | .0157                 |
| $\epsilon = .001$                                    | .2652 | .2256                 | .1433                 | .0274                 |
| $\epsilon = .01$                                     | .6043 | .7837                 | .8151                 | .6564                 |
| Classical XOR 1, $N_{\text{Total}} = 178,781,131$    |       |                       |                       |                       |
| Pulses                                               | 6     | 5-7                   | 4-8                   | 3-9                   |
| $N_{\chi}$ Cut Point                                 | 2332  | 7108                  | 11917                 | 16684                 |
| $N_S$                                                | 1179  | 3617                  | 6034                  | 8503                  |
| $\epsilon = 0$ p-value                               | .3023 | .0691                 | .0847                 | .0065                 |
| $\epsilon = .0001$                                   | .3057 | .0714                 | .0881                 | .0070                 |
| $\epsilon = .001$                                    | .3368 | .0944                 | .1239                 | .0130                 |
| $\epsilon = .01$                                     | .6730 | .5806                 | .7908                 | .5390                 |
| Classical XOR 2, $N_{\text{Total}} = 177,785,896$    |       |                       |                       |                       |
| Pulses                                               | 6     | 5-7                   | 4-8                   | 3-9                   |
| $N_{\chi}$ Cut Point                                 | 2384  | 7120                  | 11921                 | 16690                 |
| $N_S$                                                | 1215  | 3616                  | 6087                  | 8546                  |
| $\epsilon = 0$ p-value                               | .1784 | .0942                 | .0105                 | $9.54 \times 10^{-4}$ |
| $\epsilon = .0001$                                   | .1809 | .0970                 | .0111                 | .0010                 |
| $\epsilon = .001$                                    | .2050 | .1257                 | .0183                 | .0022                 |
| $\epsilon = .01$                                     | .5219 | .6451                 | .4504                 | .3013                 |
| Classical XOR 3, $N_{\text{Total}} = 182,137,032$    |       |                       |                       |                       |
| Pulses                                               | 6     | 5-7                   | 4-8                   | 3-9                   |
| $N_{\chi}$ Cut Point                                 | 2376  | 7211                  | 12127                 | 16979                 |
| $N_S$                                                | 1257  | 3800                  | 6378                  | 8820                  |
| $\epsilon = 0$ p-value                               | .0025 | $2.44 \times 10^{-6}$ | $5.85 \times 10^{-9}$ | $2.03 \times 10^{-7}$ |
| $\epsilon = .0001$                                   | .0025 | $2.64 \times 10^{-6}$ | $6.66 \times 10^{-9}$ | $2.33 \times 10^{-7}$ |
| $\epsilon = .001$                                    | .0033 | $5.40 \times 10^{-6}$ | $2.08 \times 10^{-8}$ | $7.73 \times 10^{-7}$ |
| $\epsilon = .01$                                     | .0331 | .0020                 | $2.31 \times 10^{-4}$ | .0069                 |

### 3. Equiprobability of settings.

We tested the hypothesis that Alice's settings were exactly equiprobable and that Bob's settings were exactly equiprobable. For the six experimental runs, Bob's p-values were 0.94, 0.49, 0.04, 0.27, 0.99, and 0.65, with three observed biases above  $1/2$  and three below  $1/2$ , and thus exhibited insufficient evidence to reject the null hypothesis that Bob's settings were equiprobable. Alice's p-values were 0.09, 0.07, 0.0002, 0.09, 0.11, and 0.03, and all six observed

TABLE S-II. Setting and measurement outcomes for the case of 5 aggregate pulses reported in the manuscript (Classical XOR3). From this table it is possible to calculate a variety of Bell inequalities.

|          |        | Outcomes |       |       |          |
|----------|--------|----------|-------|-------|----------|
|          |        | ++       | +0    | 0+    | 00       |
| Settings | $ab$   | 6378     | 3289  | 3147  | 44336240 |
|          | $ab'$  | 6794     | 2825  | 23230 | 44311018 |
|          | $a'b$  | 6486     | 21358 | 2818  | 44302570 |
|          | $a'b'$ | 106      | 27562 | 30000 | 44274530 |

TABLE S-III. Distribution of p-values from tests of no-signaling. The bottom row shows the number of times a p-value within the range specified by the top row was observed during 120 tests.

| Range              | 0 to 0.1 | 0.1 to 0.2 | 0.2 to 0.3 | 0.3 to 0.4 | 0.4 to 0.5 | 0.5 to 0.6 | 0.6 to 0.7 | 0.7 to 0.8 | 0.8 to 0.9 | 0.9 to 1 |
|--------------------|----------|------------|------------|------------|------------|------------|------------|------------|------------|----------|
| Number of p-values | 12       | 12         | 8          | 10         | 14         | 15         | 14         | 13         | 11         | 11       |

biases were above 1/2. This appears to be some moderate evidence that Alice's settings generator slightly favored the setting  $a$ . Alice's observed biases were, in order of experimental run, 0.500059, 0.500088, 0.500138, 0.500063, 0.500060, and 0.500080.

- 
- [S1] J. Shao, *Mathematical Statistics*, Springer Texts in Statistics (Springer, New York, 1998) See 2nd edition pages 126-127.
- [S2] J. Barrett, D. Collins, L. Hardy, A. Kent, and S. Popescu, Phys. Rev. A **66**, 042111 (2002), arXiv:quant-ph/0205016.
- [S3] R. D. Gill, in *Mathematical Statistics and Applications: Festschrift for Constance van Eeden*, Vol. 42, edited by M. Moore, S. Froda, and C. Léger (Institute of Mathematical Statistics. Beachwood, Ohio, 2003) pp. 133–154, arXiv:quant-ph/0110137.
- [S4] Y. Zhang, S. Glancy, and E. Knill, Phys. Rev. A **84**, 062118 (2011), arXiv:1108.2468.
- [S5] Y. Zhang, S. Glancy, and E. Knill, Phys. Rev. A **88**, 052119 (2013), arXiv:1303.7464.
- [S6] P. Bierhorst, J. Phys. A **48**, 195302 (2015).
- [S7] J. F. Clauser and M. A. Horne, Phys. Rev. D **10**, 526 (1974).
- [S8] P. H. Eberhard, Phys. Rev. A **47**, R747 (1993).
- [S9] M. Giustina, A. Mech, S. Ramelow, B. Wittmann, J. Kofler, J. Beyer, A. Lita, B. Calkins, T. Gerrits, S. W. Nam, R. Ursin, and A. Zeilinger, Nature **497**, 227 (2013), arXiv:1212.0533.
- [S10] P. Bierhorst, (2013), arXiv:1312.2999.
- [S11] J. Kofler and M. Giustina, (2014), arXiv:1411.4787.
- [S12] A. Fine, Phys. Rev. Lett. **48**, 291 (1982).
- [S13] The use of trade names is intended to allow the measurements to be appropriately interpreted, and does not imply endorsement by the US government, nor does it imply these are necessarily the best available for the purpose used here.
- [S14] Manual: *Electrooptical Modulator Pockels Cell Driver, Model PCD-dpp*, Bergmann Messgeräte Entwicklung KG (2008).
- [S15] C. Abellán, W. Amaya, M. Jofre, M. Curty, A. Acín, J. Capmany, V. Pruneri, and M. W. Mitchell, Opt. Express **22**, 1645 (2014), arXiv:1401.5658.
- [S16] M. W. Mitchell, C. Abellán, and W. Amaya, Phys. Rev. A **91**, 012314 (2015), arXiv:1501.02959.
- [S17] C. Abellan, W. Amaya, D. Mitrani, V. Pruneri, and M. W. Mitchell, ArXiv e-prints (2015), arXiv:1506.02712 [quant-ph].
- [S18] A. Rukhin, J. Soto, J. Nechvatal, M. Smid, E. Barker, S. Leigh, M. Levenson, M. Vangel, D. Banks, A. Heckert, J. Dray, and S. Vo, *A Statistical Test Suite for Random and Pseudorandom Number Generators for Cryptographic Applications*, Tech. Rep. 800-22 (National Institute of Standards and Technology, 2010).
- [S19] P. L'Ecuyer and R. Simard, ACM Trans. Math. Softw. **33**, 22 (2007).
- [S20] A. Einstein, Deutsche Physikalische Gesellschaft **18**, 318 (1916).
- [S21] R. G. Brown, Access available at [http://csrc.nist.gov/groups/ST/toolkit/rng/documentation\\_software.html](http://csrc.nist.gov/groups/ST/toolkit/rng/documentation_software.html) (2004).
- [S22] J. Walker, "Ent: A pseudorandom number sequence test program (2008)," Access available at <http://www.fourmilab.ch/random/>.
